# Supplementary material for: Rethinking Bradley-Terry Models in Preference-Based Reward Modeling: Foundations, Theory, and Alternatives
Source: arXiv:2411.04991 source file (2025-01-26)
Supplement: Supplementary file 1 [file appendix.tex]

\newpage
\appendix
\section{Underlying Assumptions of Applying the Bradley-Terry Model in Preference Annotations}
\label{appdx:implication_of_assumptions}
%\ys{can we say this is rederiving this model from cognitive bottle neck or something indicating we start from human bias rather than random game?}
Different from those prior works that challenge the \textit{practical application} of the BT model~\cite{azar2023general,munos2023nash,tang2024generalized}, we revisit the basic assumptions of modeling human preference annotations with the BT model, and answer the following questions:

\textbf{\textit{What are the underlying assumptions when we assume the BT model can be used to model the preference annotations?}}

The canonical interpretation of how to apply \eqref{eqn:BT} in preference-based learning is that: when randomly sampling a human annotator from the population, the human annotator's choice of the preferred response is proportional to the response's utility value. Formally, we use $\prompt, \response_1,\response_2$ to denote the prompt and responses, the above interpretation implies the following assumptions:
\begin{assumption}[Existence of a Deterministic Oracle Utility Value]
    Given $\prompt$, the utility value of any response $\response$ exists and is deterministic. i.e., $\truereward_{\prompt,\response}, \forall \prompt,\response$ is a deterministic real value.
\end{assumption}
\begin{comment}
\begin{definition}[Individual Utility Evaluation Bias]
    For a \textbf{random} human annotator $A$, their evaluation of the utility value will deviate from the oracle utility value according to their individualized bias:
    \begin{equation}
        \truereward^{(A)}_{\prompt,\response} = \truereward_{\prompt,\response} + \annotatorbias(\prompt,\response,A),
    \end{equation}
    where $\annotatorbias(\prompt,\response,A)$ is a function over prompt $\prompt$, response $\response$, and annotator-dependent. Furthermore, we have 
    \begin{equation}
        \mathbb{E}_A \left[ \annotatorbias(\prompt,\response,A) \right] = 0, \forall \prompt,\response,
    \end{equation}
    and therefore
    \begin{equation}
        \mathbb{E}_A \left[ \truereward^{(A)}_{\prompt,\response} \right] = \truereward_{\prompt,\response}, \forall \prompt,\response,
    \end{equation}
\end{definition}
\ys{Note to self: this might not be compatible with logistic difference assumption}
\end{comment}
\begin{definition}[Individual Annotation under Bias]
    For annotator $A$, the annotation result is deterministic and depends on the comparison of their biased evaluation of the utility values of both responses $\response_1$ and $\response_2$, according to 
    \begin{equation}
        P_A(\response_1\succ \response_2 | \prompt) = \mathbbm{1}(\truereward^{(A)}_{\prompt,\response_1} > \truereward^{(A)}_{\prompt,\response_2}) = \mathbbm{1}\bigl(\truereward_{\prompt,\response_1} -\truereward_{\prompt,\response_2}  > \annotatorbias(\prompt,\response_1,A) - \annotatorbias(\prompt,\response_2,A) \bigr)
    \end{equation}
\end{definition}
Based on the above definitions, we can now explicitly write the assumption of applying the BT model to this randomized annotation process:
\begin{assumption}[Logistic Difference Assumption]
    The $\annotatorbias(\prompt,\response_1,A) - \annotatorbias(\prompt,\response_2,A)$ is sampled iid from a standard logistic distribution for all $\prompt,\response,A$:
    \begin{equation}
        P(\annotatorbias(\prompt,\response_1,A) - \annotatorbias(\prompt,\response_2,A) \le t) = \frac{1}{1+e^{-t}}
    \end{equation}
\end{assumption}
\begin{remark}(Transitive property of difference)
    A reader might be (rightfully) worried if this assumption is consistent with transitive property of difference, e.g., when considering multiple comparisons we have to have $\annotatorbias(\prompt,\response_{1},A)-\annotatorbias(\prompt,\response_3,A)=\annotatorbias(\prompt,\response_{1},A)-\annotatorbias(\prompt,\response_{2},A) + \annotatorbias(\prompt,\response_{2},A)-\annotatorbias(\prompt,\response_3,A)$ while knowing sum of (independent) logistic distributions is not logistic. One should be aware that the two terms being summed are not independent and the assumption can be achieved by assuming all annotator biases are independently Gumbel distributed with the same scale parameter.   
\end{remark}
With this assumption, we arrive at the BT-\textit{type} model
\begin{proposition}[BT-\textit{type} Model on Annotation under Logistic Difference Assumption]
    \begin{equation}
        P(\response_{1}\succ \response_{2} | \prompt) = P\bigl(\truereward_{\prompt,\response_{1}} -\truereward_{\prompt,\response_{2}}  > \annotatorbias(\prompt,\response_1,A) - \annotatorbias(\prompt,\response_2,A) \bigr) = \frac{1}{1+ e^{-(\truereward_{\prompt,\response_{1}} -\truereward_{\prompt,\response_{2}})}}
    \end{equation}
\end{proposition}
In comparison, we can alternatively have the following assumption and have another model:
\begin{assumption}[Gaussian Difference Assumption]
    The $\annotatorbias(\prompt,\response_1,A) - \annotatorbias(\prompt,\response_2,A)$ is sampled from a standard Gaussian distribution:
    \begin{equation}
        \annotatorbias(\prompt,\response_1,A) - \annotatorbias(\prompt,\response_2,A)\sim \mathcal{N}(0,1)
    \end{equation}
\end{assumption}
\begin{proposition}[Model on Annotation under Gaussian Difference Assumption]
    \begin{equation}
        P(\response_{1}\succ \response_{2} | \prompt) = P\bigl(\truereward_{\prompt,\response_{1}} -\truereward_{\prompt,\response_{2}}  > \annotatorbias(\prompt,\response_1,A) - \annotatorbias(\prompt,\response_2,A) \bigr) = \Phi(\truereward_{\prompt,\response_{1}} -\truereward_{\prompt,\response_{2}}),
    \end{equation}
    where $\Phi$ is the CDF of the Gaussian distribution.
\end{proposition}
%\begin{remark}(Assumption Self-Consistency)
%    We denote that this Gaussian difference assumption is self-consistent, and one way to achieve it is by having biases being Gaussian.
%\end{remark}
The next paragraph elaborates implications of those different assumptions.

\paragraph{Understanding the BT Model from a Gaussian Assumption on Players' Performance in a Game}
Technically, the BT model assumes that a player's ability \textbf{in a specific game} can be represented by a score. To better understand the rationale behind the BT model, we can take a step back and consider a Gaussian assumption for game performances. Specifically, we assume that in each two-player game, a player's performance can be modeled as a Gaussian distribution centered on their score, with the variance of these distributions capturing the stochastic nature of the game and the variability in the players' performances.

For instance, when player $A$ with a score of $S_A$ and variance $\sigma_A$ competes against player $B$ with a score of $S_B$ and variance $\sigma_B$, the probability that $A$ defeats $B$ in a game (denoted as $A \succ B$), given the Gaussian assumption on performance, is
\begin{equation}
\label{eqn:bt_prob}
    P(A \succ B) =P\left(x_a \ge x_b | x_a\sim N(S_A, \sigma_A^2), x_b\sim N(S_B, \sigma_B^2)\right) = \frac{1}{2} + \frac{1}{2}\mathrm{erf}\left(\frac{S_A-S_B}{\sqrt{2(\sigma_A^2+\sigma_B^2)}}\right).
\end{equation}
This is known to be the Thurstonian model~\citep{thurstone1927law}. In practice, if we further \textbf{assume} that the stochasticity characterized by performance variance is game-dependent rather than player-dependent, the denominator in \eqref{eqn:bt_prob} becomes a player-agnostic constant, which can be absorbed into the players' scores. In other words, \textbf{the absolute values in the scoring system are scaled by the inherent variability of the game.}

In the BT model, the $\mathrm{tanh}(\cdot)$ rather than the error function $\mathrm{erf}(\cdot)$ is used, for the sake of a better empirical fit and mathematical convenience.\footnote{So equivalently, the BT model assumes the players' performance differences are sampled from a logistic distribution rather than a Gaussian distribution.} Formally, the BT model is 
\begin{equation}
    \label{eqn:bt-model}
    P(A\succ B) = \frac{1}{1+e^{-(S_A - S_B)}}
\end{equation}

\section{Implication of Different Assumptions}
\paragraph{Understanding the Bradley-Terry Model from a Gaussian Assumption on Players' Performance in a Game}
\label{appdx:implication_of_assumptions}
Technically, the Bradley-Terry model assumes that a player's ability \textbf{in a specific game} can be represented by a score. To better understand the rationale behind the Bradley-Terry model, we can take a step back and consider a Gaussian assumption for game performances. Specifically, we assume that in each two-player game, a player's performance can be modeled as a Gaussian distribution centered on their score, with the variance of these distributions capturing the stochastic nature of the game and the variability in the players' performances.

For instance, when player $A$ with a score of $S_A$ and variance $\sigma_A$ competes against player $B$ with a score of $S_B$ and variance $\sigma_B$, the probability that $A$ defeats $B$ in a game (denoted as $A \succ B$), given the Gaussian assumption on performance, is
\begin{equation}
\label{eqn:bt_prob}
    P(A \succ B) =P\left(x_a \ge x_b | x_a\sim N(S_A, \sigma_A^2), x_b\sim N(S_B, \sigma_B^2)\right) = \frac{1}{2} + \frac{1}{2}\mathrm{erf}\left(\frac{S_A-S_B}{\sqrt{2(\sigma_A^2+\sigma_B^2)}}\right).
\end{equation}
This is known to be the Thurstonian model~\citep{thurstone1927law}. In practice, if we further \textbf{assume} that the stochasticity characterized by performance variance is game-dependent rather than player-dependent, the denominator in \eqref{eqn:bt_prob} becomes a player-agnostic constant, which can be absorbed into the players' scores. In other words, \textbf{the absolute values in the scoring system are scaled by the inherent variability of the game.}

In the Bradley-Terry model, the $\mathrm{tanh}(\cdot)$ rather than the error function $\mathrm{erf}(\cdot)$ is used, for the sake of a better empirical fit and mathematical convenience.\footnote{So equivalently, the Bradley-Terry model assumes the players' performance differences are sampled from a logistic distribution rather than a Gaussian distribution.} Formally, the Bradley-Terry model is 
\begin{equation}
    \label{eqn:bt-model}
    P(A\succ B) = \frac{1}{1+e^{-(S_A - S_B)}}
\end{equation}

\section{Missing Proofs}
\subsection{Proof of Theorem~\ref{theorem:1.1} (See page~\pageref{theorem:1.1})}
\TheoremOne*
\begin{proof}
Given the over-parametrization issue (adding a constant to all \(S_i\) leaves the model unchanged), we can set the first parameter (e.g., \(S_1 = 0\)) to identify the model. To find the MLEs, we take the partial derivatives of the log-likelihood function with respect to each \(S_i\) and set them to zero. The partial derivative of the log-likelihood function with respect to \(S_i\) is given by:
\begin{equation}
\frac{\partial \ell_M(\mathbf{S})}{\partial S_i} = \frac{\partial \ell_M(S_1, S_2, \dots, S_k)}{\partial S_i} = \sum_{m : i_m = i} \left[H_m - \frac{e^{S_i - S_{j_m}}}{1 + e^{S_i - S_{j_m}}}\right] - \sum_{m : j_m = i} \left[H_m - \frac{e^{S_{i_m} - S_i}}{1 + e^{S_{i_m} - S_i}}\right]
\end{equation}
There are $k-1$ parameters to estimate and $k-1$ equations. Moreover, we have 
the log-likelihood function \( \ell_M(\mathbf{S}) \) to be concave in \( \mathbf{S} \), as the Hessian matrix \( H_M(\mathbf{S}) \) is negative semi-definite:
\begin{equation}
H_M(\mathbf{S}) = \frac{\partial^2 \ell_M(\mathbf{S})}{\partial \mathbf{S} \partial \mathbf{S}^\top} \preceq 0.
\end{equation}
This concavity ensures that \( \ell_M(\mathbf{S}) \) has a unique global maximum.

We use \( \mathbf{S}^* \) to denote the maximizer of the expected log-likelihood function. %\( \mathbf{S}^* \) is the unique point where the expected log-likelihood attains its maximum.
As \( M \) increases, the empirical distribution of the pairwise comparisons \( (H_m, i_m, j_m) \) will converge almost surely to the true distribution of the pairwise comparisons according to the Law of Large Numbers. This implies that the empirical log-likelihood function \( \ell_M(\mathbf{S}) \) converges almost surely to the expected log-likelihood function \( \mathbb{E}[\ell_M(\mathbf{S})] \) as \( M \to \infty \).

The expected log-likelihood function \( \mathbb{E}[\ell_M(\mathbf{S})] \) is concave, as indicated by the negative semi-definiteness of the Hessian matrix \( H_M(\mathbf{S}) \). Because of the strict concavity, there is a unique maximum of the expected log-likelihood at the true parameter values \( \mathbf{S}^* \).

\textit{\textbf{Proof 1:}} \hs{@ys: which one do you think is better?}
\ys{None. It's very likely proven somewhere and the proofs here as written are not quite there yet. cite \citet{simons1999asymptotics} for some high dimensional results \citet{han2020asymptotic} for some sparse cases (when the number of players also diverge), for fixed number of teams the results might follow classic MLE theory. I'd say we better find some references rather than proof ourselves since it should involve some technical assumptions esp. on identifiability side (things are only identified up to a constant) \citet{ford1957solution} had some discussion on this, \citet{duchi2013asymptotics} might be a good reference on this type of models in general.}
\jef{@YS Do you think the above can be proved strictly by citing existing paper? if yes we should try to understand them and simply apply them in our setting. Can you think of a rough outline of the proof in the above setting? Also what part do you think is missing in @HS proof atm? I am not very good with theory so would like to hear your thoughts on this.}

Suppose that the MLE \( \hat{\mathbf{S}}_M \) is not consistent. Then, there exists an \( \epsilon > 0 \) such that:
\begin{equation}
\limsup_{M \to \infty} P\left( \|\hat{\mathbf{S}}_M - \mathbf{S}^*\| > \epsilon \right) > 0.
\end{equation}
This means that with positive probability, the estimator \( \hat{\mathbf{S}}_M \) lies outside the ball \( B(\mathbf{S}^*, \epsilon) \) centered at \( \mathbf{S}^* \) with radius \( \epsilon \).

Consider any point \( \mathbf{S}' \) in the complement of \( B(\mathbf{S}^*, \epsilon) \), i.e., \( \mathbf{S}' \notin B(\mathbf{S}^*, \epsilon) \). Because \( \ell(\mathbf{S}) \) is strictly concave and maximized at \( \mathbf{S}^* \), we have:
\begin{equation}
\ell(\mathbf{S}') < \ell(\mathbf{S}^*).
\end{equation}
Since \( \frac{1}{M} \ell_M(\mathbf{S}) \) converges uniformly to \( \ell(\mathbf{S}) \), for sufficiently large \( M \), the empirical log-likelihood function \( \ell_M(\mathbf{S}) \) will also satisfy:
\begin{equation}
\ell_M(\mathbf{S}') < \ell_M(\mathbf{S}^*).
\end{equation}
This implies that for large enough \( M \), the MLE \( \hat{\mathbf{S}}_M \), which maximizes \( \ell_M(\mathbf{S}) \), cannot lie outside \( B(\mathbf{S}^*, \epsilon) \) because \( \ell_M(\mathbf{S}') \) would be strictly less than \( \ell_M(\mathbf{S}^*) \).

However, this contradicts the assumption that \( \hat{\mathbf{S}}_M \) does not converge to \( \mathbf{S}^* \). Therefore, our initial supposition must be false, and we conclude:
\begin{equation}
\lim_{M \to \infty} P\left( \|\hat{\mathbf{S}}_M - \mathbf{S}^*\| > \epsilon \right) = 0 \quad \text{for all } \epsilon > 0,
\end{equation}
which means that \( \hat{\mathbf{S}}_M \xrightarrow{P} \mathbf{S}^* \) as \( M \to \infty \).

\textit{\textbf{Proof 2:}} \hs{@ys: which one do you think is better?}

By the Maximum Likelihood Principle, \( \hat{\mathbf{S}}_M \) is the maximizer of the empirical log-likelihood function. Since the empirical log-likelihood function converges to the expected log-likelihood function, and the expected log-likelihood function has a unique maximum at \( \mathbf{S}^* \), the sequence \( \hat{\mathbf{S}}_M \) must converge to \( \mathbf{S}^* \) as \( M \to \infty \).

Formally, for any \( \epsilon > 0 \) and \( \delta > 0 \), there exists an \( M_0 \) such that for all \( M > M_0 \),
\begin{equation}
P\left( \|\hat{\mathbf{S}}_M - \mathbf{S}^*\| > \epsilon \right) < \delta,
\end{equation}
which implies that \( \hat{\mathbf{S}}_M \xrightarrow{P} \mathbf{S}^* \) as \( M \to \infty \).

To prove consistency, consider the probability that \( \hat{\mathbf{S}}_M \) deviates from the true parameter \( \mathbf{S}^* \) by more than \( \epsilon > 0 \):
\begin{equation}
P\left(\|\hat{\mathbf{S}}_M - \mathbf{S}^*\| > \epsilon \right).
\end{equation}
Assume \( \hat{\mathbf{S}}_M \) does not converge to \( \mathbf{S}^* \). Then, for some \( \mathbf{S}' \notin B(\mathbf{S}^*, \epsilon) \), we would have \( \ell_M(\mathbf{S}') \geq \ell_M(\mathbf{S}^*) \).
By the uniform convergence established above, and since \( \mathbf{S}^* \) is the unique maximizer of \( \ell(\mathbf{S}) \), the probability that \( \ell_M(\mathbf{S}') \geq \ell_M(\mathbf{S}^*) \) tends to zero as \( M \) increases. Therefore, the probability that \( \hat{\mathbf{S}}_M \) lies outside \( B(\mathbf{S}^*, \epsilon) \) also tends to zero:
\begin{equation}
P\left(\|\hat{\mathbf{S}}_M - \mathbf{S}^*\| > \epsilon \right) \xrightarrow{M \rightarrow \infty} 0.
\end{equation}
Thus, \( \hat{\mathbf{S}}_M \xrightarrow{P} \mathbf{S}^* \), proving that the MLE is consistent.
\end{proof}

\subsection{Proof of Proposition~\ref{prop:1} (See page~\pageref{prop:1})}
\label{appdx:proof_prop1}
\PropAvgQuality*
% \proof 
% Leveraging the linearity of operator $\boldsymbol{l}$, the definition of the operator norm $||\cdot||_\mathrm{op}$, and Definition~\ref{def:belief_corpus_residual}, we have:
% \begin{equation}
%     \begin{split}
%         ||\boldsymbol{l}(\hat{b}) - \boldsymbol{l}(b_t)||_\mathcal{V} &= ||\boldsymbol{l}(\hat{b} - b_t)||_\mathcal{V} \\
%         &\le ||\boldsymbol{l}||_\mathrm{op}\cdot ||\hat{b} - b_t||_\mathcal{V} \\
%         &= ||\boldsymbol{l}||_{\mathrm{op}} \cdot r_\mathcal{C}(b_t)
%     \end{split}
% \end{equation}
% \endproof

\begin{proof}
    To get the PDF of $f(\tau)$, denote $\tau = \sigma(|\rho|)$, where we use $\rho(x) = \beta(r^*(y_1|x) - r^*(y_2|x))$, we have $\rho(x) \sim \mathcal{N}(0,2\beta^2\sigma_x^2)$ follows the normal distribution, and $|\rho(x)|$ follows a folded normal distribution, its cumulative distribution function, mean and variance are given by
    \begin{equation}
        F_{|\rho|}(x; \mu=0, \sigma^2 = 2\beta^2\sigma_x^2) = \mathrm{erf}\left(\frac{x}{2\beta\sigma_x}\right), ~~ \mu_{|\rho|} = \frac{2\beta\sigma_x}{\sqrt{\pi}}, ~~ \sigma_{|\rho|}^2 = 2\beta^2\sigma_x^2(1-\frac{2}{\pi}),
    \end{equation}
    respectively. 
    
To find the PDF of \( \tau = \sigma(|\rho|) \), we use the change of variables formula. If \( Y = g(X) \) and \( g \) is a monotonic function, the PDF of \( Y \), \( f_Y(y) \), can be obtained by:
\begin{equation}
    f_Y(y) = f_X(g^{-1}(y)) \left| \frac{d}{dy} g^{-1}(y) \right|.
\end{equation}

For the sigmoid function, the inverse is given by:
\begin{equation}
    g^{-1}(y) = \log\left(\frac{y}{1-y}\right).
\end{equation}

The derivative of the inverse sigmoid function is:
\begin{equation}
    \frac{d}{dy} g^{-1}(y) = \frac{1}{y(1-y)}.
\end{equation}

Plugging these into the change of variables formula, we get:
\begin{equation}
    f_\tau(t) = \frac{1}{\sqrt{\pi \beta^2\sigma_x^2}} \exp\left(-\frac{\left(\log\left(\frac{t}{1-t}\right)\right)^2}{4\beta^2\sigma_x^2}\right) \cdot \frac{1}{t(1-t)}.
\end{equation}
This completes the proof.
\end{proof}

\subsection{Proof of Theorem \ref{theorem1} (See Page \pageref{theorem1})}
\label{appdx:proof_theorem1}

\ThmO*

\begin{proof}
The idea of the proof is to first use Markov's inequality to bound probability that for a given distance $\Delta r$ the preference model not well approximate the annotator and under the event that the preference model approximate the annotator well, we bound the total error combined by preference model and annotator. 

By assumption we have the (marginal) error probability averaging over all distances $r$ is 

\begin{equation}
\begin{split}
    &\mathbb{P}_{x, y_1,y_2 \sim \ell(x)} \left[ \mathbbm{1}\left(\sign \hat{H}_\theta(x, y_1, y_2)\ne \sign \mathcal{H}_\beta (x, y_1, y_2)\right) \right]\\
        =&\E_{r} \left[ \mathbb{P}\left( \sign \hat{H}_\theta(x, y_1, y_2)\ne \sign \mathcal{H}_\beta (x, y_1, y_2)    \bigg|  \Delta r \right) \right]\\
        <& \delta\epsilon
\end{split}
\end{equation}
Denote that
\begin{equation}
    \Pi_r:=\mathbb{P}\left( \sign \hat{H}_\theta(x, y_1, y_2)\ne \sign \mathcal{H}_\beta (x, y_1, y_2)    \bigg|  \Delta r \right)
\end{equation}

%Since this is a random variable within $(0,1)$, we have $\E \Pi_r \ge \E \Pi_r^2$, thus $var(\Pi_r)=\E \Pi_r^2-(\E\Pi_r)^2\le \E\Pi_r<\epsilon$.

%By Chebyshev, we have 
%\begin{align*}
%    \mathbb{P}_{r}\left( \Pi_r\ge \epsilon  \right)\le \mathbb{P}_{r}\left( \Pi_r\ge \epsilon/2 + \E \Pi_r  \right)
%\end{align*}

by Markov's inequality
\begin{align}
    &\mathbb{P}_{r}\left( \Pi_r\ge \epsilon  \right)\le \frac{\delta\epsilon}{\epsilon} = \delta
\end{align}
In the event  $\{\Delta r: \mathbb{P}\left( \sign \hat{H}_\theta(x, y_1, y_2)\ne \sign \mathcal{H}_\beta (x, y_1, y_2)    \bigg|  \Delta r \right)<\epsilon\}$, with probability $1-\delta$ we bound the error rate as function of $\Delta r$.
Condition on $\Delta r$, define the following probabilities:
\begin{itemize}
    \item \( p_{\text{annotator}} = \sigma(\beta \Delta r) \) is the probability that the annotator \(\mathcal{H}_\beta\) is correct (i.e., agrees with the oracle utility) given the oracle distance.
    \item \( 1 - p_{\text{annotator}} = 1 - \sigma(\beta \Delta r) \) is the probability that the annotator \(\mathcal{H}_\beta\) is incorrect given the oracle distance.
\end{itemize}

Given the bounded difference between $\hat{H}_\theta$ and $H_\beta$:
\begin{itemize}
    \item Correct Case: When the annotator is correct, the learned model agrees with the annotator with probability at least \( 1 - \epsilon \). Thus:
    \begin{equation}
    p_{\text{correct}} \geq (1 - \epsilon) \cdot \sigma(\beta \Delta r).
    \end{equation}
    \item Incorrect Case: When the annotator is incorrect, the learned model agrees with the annotator with probability at most \( \epsilon \). Thus:
    \begin{equation}
    p_{\text{incorrect}} \leq \epsilon \cdot (1 - \sigma(\beta \Delta r)).
    \end{equation}
\end{itemize}

The order consistency of the learned model \(\hat{H}_{\theta^*}\) with the oracle utility can be expressed as:
\begin{equation}
\mathbb{E}_{x, y_1, y_2 \sim \ell(x)}\left[\mathbbm{1}\left(\hat{H}_{\theta^*}(x, y_1, y_2)(r^*(y_1|x) - r^*(y_2|x)) \geq 0\right)\bigg|  \Delta r\right] = p_{\text{correct}} \cdot p_{\text{annotator}} + p_{\text{incorrect}} \cdot (1 - p_{\text{annotator}}).
\end{equation}

Substituting the bounds and simplifying, we have
\begin{equation}
\mathbb{E}_{x, y_1, y_2 \sim \ell(x)}\left[\mathbbm{1}\left(\hat{H}_{\theta^*}(x, y_1, y_2)(r^*(y_1|x) - r^*(y_2|x)) \geq 0\right)\bigg|  \Delta r\right]\geq (1 - \epsilon) \cdot \sigma^2(\beta \Delta r) + \epsilon \cdot (1 - \sigma(\beta \Delta r))^2.
\end{equation}

%Further if we assume that with probability at least $1-\kappa$, that $\sigma(\beta \Delta r)\ge \sqrt{\epsilon^2+1-(\xi - \epsilon)}+\epsilon$ with $3/4-\epsilon>\xi > 3\epsilon$ implies $(1 - \epsilon) \cdot \sigma^2(\beta \Delta r) + \epsilon \cdot (1 - \sigma(\beta \Delta r))^2 \ge 1-\xi$, the stated bound fail either 1) $\mathbb{P}_{r}>\epsilon$, with probability less than $\delta$ or 2) $\sigma(\beta \Delta r)< \sqrt{\epsilon^2+1-(\xi - \epsilon)}+\epsilon$ with probability at most $\kappa$, thus the stated bound is true with probability at least $1-\kappa-\delta$

Second part of the proof is by observing that $\sigma(\beta \Delta r)\ge \sqrt{\epsilon^2+1-3\epsilon}+\epsilon$ implies $(1 - \epsilon) \cdot \sigma^2(\beta \Delta r) + \epsilon \cdot (1 - \sigma(\beta \Delta r))^2 \ge 1-4\epsilon$ when $\epsilon<3/20$, consider this conditional bound 
\begin{align}
    \mathbb{E}_{x, y_1, y_2 \sim \ell(x)}\left[\mathbbm{1}\left(\hat{H}_{\theta^*}(x, y_1, y_2)(r^*(y_1|x) - r^*(y_2|x)) \geq 0\right)  \bigg|  \Delta r\right]\geq 1-4\epsilon
\end{align}

the stated bound fail either 1) $\Pi_{r}>\epsilon$, with probability at most $\delta$ or 2) $\sigma(\beta \Delta r)< \sqrt{\epsilon^2+1-3\epsilon}+\epsilon$ with probability at most $\kappa$, thus the stated bound is true with probability at least $1-\kappa-\delta$ due to union bound on failure modes.

Then by definition of conditional probability, the bound in theorem true.

%then with probability at least $1-\kappa-\delta$, we have 
%\begin{align*}
%    \mathbb{E}_{x, y_1, y_2 \sim \ell(x)}\left[\mathbbm{1}\left(\hat{H}_{\theta^*}(x, y_1, y_2)(r^*(y_1|x) - r^*(y_2|x)) \geq 0\right)\right]\geq 1-\xi
%\end{align*}

%The proof is completed.

\end{proof}
